# Supplementary material for: AT2: Asynchronous Trustworthy Transfers
Source: arXiv:1812.10844 source file (2019-03-05)
Supplement: Supplementary file 1 [file gossip-analysis.tex]

%!TEX root = ../../main.tex

\section{Full analysis: \erg}
\label{appendix:erganalysis}

In this appendix, we evaluate the security and complexity of \erg.

\subsection{Security}

We start by verifying that \erg\ satistifes both \textbf{no duplication}, \textbf{integrity} and $0$-\textbf{validity}, independently of $G$.

\begin{theorem}
\label{theorem:ergnoduplication}
\erg\ satisfies no duplication.
\begin{proof}
Procedure $dispatch$ explicitly checks (\cref{line:ergcheckdelivered}) if the variable $delivered$ is equal to $\bot$ before delivering any message. Before a message is delivered (\cref{line:ergdeliver}), $delivered$ is updated to a value different from $\bot$ (\cref{line:ergsetdelivered}). Therefore a correct process only delivers one message.
\end{proof}
\end{theorem}

\begin{theorem}
\label{theorem:ergintegrity}
\erg\ satistifes integrity.
\begin{proof}
Upon receiving a {\tt Gossip} message, a correct process checks its $signature$ against the public key of the designated sender $\sigma$ (\cref{line:ergchecksignature}). Moreover, if $\sigma$ is correct, it only signs $message$ when broadcasting (\cref{line:ergbroadcast}). Since we assume that cryptographic signatures cannot be forged, this implies that the message was previously broadcast by $\sigma$.
\end{proof}
\end{theorem}

\begin{theorem}
\label{theorem:ergvalidity}
\erg\ satisfies 0-validity.
\begin{proof}
Upon broadcasting a message $m$, a correct sender calls the procedure $dispatch(m, sign(m))$ (\cref{line:ergbroadcast}). Since $delivered$ is initialized to $\bot$, this immediately results in the delivery of $m$ (\cref{line:ergdeliver}).

Since the validity property is satisfied deterministically, \erg\ satisfies  $\epsilon$-validity for $\epsilon = 0$.
\end{proof}
\end{theorem}

We now compute, given the parameter $G$, the $\epsilon$-\textbf{totality} of \erg. To this end, we first prove some preliminary lemmas.

\begin{lemma}
\label{lemma:gossipreciprocation}
Let $\rho$ and $\pi$ be two correct processes, let $\rho$ be in $\pi$'s gossip sample. Then $\pi$ is eventually in $\rho$'s gossip sample.
\begin{proof}
A gossip sample is updated only upon initialization (\cref{line:erginitializesample}) or when a {\tt GossipSubscribe} message is received (\cref{line:ergupdatesample}).

If $\pi$ selected $\rho$ upon initialization, then it also sent it a {\tt GossipSubscribe} message (\cref{line:ergsubscribe}). Since Byzantine network scheduling can only finitely delay the messages between correct processes, $\rho$ eventually receives $\pi$'s message (\cref{line:ergreceivesubscribe}) and adds $\pi$ to its gossip sample.

If $\pi$ received a {\tt GossipSubscribe} message from $\rho$, then (\cref{line:ergsubscribe}) $\rho$ selected $\pi$ upon initialization, which means that $\pi$ is already in $\rho$'s gossip sample.
\end{proof}
\end{lemma}

\begin{definition}[Correct gossip network]
Let $\pi$, $\rho$ be two correct processes, let $\pi \leftrightarrow \rho$ denote the condition \emph{$\rho$ is eventually in $\pi$'s gossip sample}. \cref{lemma:gossipreciprocation} proves that
\begin{equation*}
    \rp{\pi \leftrightarrow \rho} \Leftrightarrow \rp{\rho \leftrightarrow \pi}
\end{equation*}

We define \textbf{correct gossip network} to be the undirected graph
\begin{equation}
    \mathbb{G} = \rp{\Pi_C, \cp{\rp{\pi, \rho} \in \Pi^2_C \mid \pi \leftrightarrow \rho}}
\end{equation}
\end{definition}

\begin{lemma}
\label{lemma:gossipconnectedness}
If the correct gossip network is connected, then \erg\ satisfies totality.
\begin{proof}
We start by noting that a correct process eventually delivers a message (\cref{line:ergdeliver}) if and only if it eventually sets $delivered$ to a value different from $\bot$ (\cref{line:ergsetdelivered}).

Let $\pi$ be a correct process for which eventually $delivered \neq \bot$. Upon setting $delivered \leftarrow (m \neq \bot)$, $\pi$ sends $m$ to all the processes in its gossip sample (\cref{line:ergforward}). Moreover, upon receiving a {\tt GossipSubscribe} message \emph{after} setting $delivered \leftarrow m$, $\pi$ replies with $m$ (\cref{line:ergcatchup}).

Therefore, every correct process that is eventually in $\pi$'s gossip sample eventually satisfies $delivered \neq \bot$. If $\mathbb{G}$ is connected, then a path exists in $\mathbb{G}$ between $\pi$ and every other correct process, and they all eventually satisfy $delivered \neq \bot$, i.e., they deliver a message.
\end{proof}
\end{lemma}

From \cref{lemma:gossipconnectedness} it follows that \erg\ satisfies $\epsilon$-totality if the probability of $\mathbb{G}$ being disconnected is at most $\epsilon$.

\begin{lemma}
\label{lemma:gossipconnectionprobability}
In the limit $N \rightarrow \infty$, $\mathbb{G}$ is a $G\rp{C, p}$ Erdős–Rényi graph, with
\begin{equation*}
    p = 1 - \rp{1 - \frac{G}{N}}^2
\end{equation*}
\begin{proof}
It is a known result that, for large samples and small probabilities, a binomial distribution converges to a Poisson distribution:
\begin{equation*}
    \lim_{\substack{N \rightarrow \infty \\ Np = \text{const}}} \qp
    {
        \bin{N}{p}{n} = {N \choose n} p^n \rp{1 - p}^{N - n}
    }
    =
    \qp
    {
        \frac{\rp{Np}^n}{n!}e^{-Np} = \pois{Np}{n}
    }
\end{equation*}
therefore, in the limit $N \rightarrow \infty$,
\begin{equation}
    \label{equation:poissontobinomial}
    \pois{G}{n} \simeq \bin{N}{\frac{G}{N}}{n}
\end{equation}

As we discussed in \cref{subsection:ergalgorithm}, a gossip sample $\mathcal{G}$ is initialized upon initialization (\cref{line:erginitializesample}) by first sampling a value $\bar G$ from a $\text{Pois}\qp{G}$ distribution, then selecting $\bar G$ distinct processes from $\Pi$ with uniform probability.

Let $\pi \in \Pi_C, \rho \in \Pi$, let $\mathcal{G}^{in}_\pi$ be $\pi$'s initial gossip sample, let $q = G/N$. By the law of total probability, and using \cref{equation:poissontobinomial}, we have for large $N$
\begin{eqnarray*}
\prob{\rho \in \mathcal{G}^{in}_\pi} &=& \sum_{\bar G = 0}^N \rp{\prob{\rho \in \mathcal{G}^{in}_\pi \mid \bar G} \prob{\bar G}} = \\
&=& \sum_{\bar G = 0}^N \rp{\frac{\bar G}{N} \pois{G}{\bar G}} \simeq \sum_{\bar G = 0}^N \rp{\frac{\bar G}{N} \bin{N}{q}{\bar G}} = \\
&=& \sum_{\bar G = 0}^N \rp{\frac{\bar G}{N} {N \choose {\bar G}} q^{\bar G}\rp{1 - q}^{N - \bar G}} = \\
&=& \sum_{\bar G = 0}^N \rp{\frac{\bar G}{N} \frac{N!}{\bar G! \rp{N - \bar G}!} q^{\bar G} \rp{1 - q}^{N - \bar G}} = \\
&=& \sum_{\bar G = 1}^N \rp{\frac{\rp{N - 1}!}{\rp{\bar G - 1}!\rp{N - \bar G}!} q q^{\bar G - 1}\rp{1 - q}^{N - \bar G}} = \\
&=& q \sum_{\bar G' = 0}^{N - 1} \rp{\frac{\rp{N - 1}!}{\bar G'! \rp{N - 1 - \bar G'}!} q^{\bar G'} \rp{1 - q}^{N - 1 - \bar G'}} = \\
&=& q \sum_{\bar G' = 0}^{N - 1} \bin{N - 1}{q}{\bar G'} = q
\end{eqnarray*}

Let $\rho_1, \ldots, \rho_R$ be distinct processes, with $R \leq N$. Similar calculations yield
\begin{equation}
    \label{equation:independentgossipsampling}
    \prob{\rho_1 \in \mathcal{G}^{in}_\pi, \ldots, \rho_R \in \mathcal{G}^{in}_\pi} = q^R
\end{equation}

\cref{equation:independentgossipsampling} proves that every process $\rho \in \Pi$ has an independent probability $q$ of being in $\mathcal{G}^{in}_\pi$. Since for any two $\pi, \xi \in \Pi_C$ we have
\begin{equation*}
    \rp{\pi \leftrightarrow \xi} \Leftrightarrow \rp{\pi \in \mathcal{G}^{in}_\xi \vee \xi \in \mathcal{G}^{in}_\pi}
\end{equation*}
we can derive the probability $p$ of any two correct processes being connected:
\begin{equation}
    \label{equation:gossipconnectionprobability}
    p = 1 - \rp{1 - q}^2 = 1 - \rp{1 - \frac{G}{N}}^2
\end{equation}

Therefore, following \cref{equation:independentgossipsampling,equation:gossipconnectionprobability}, $\mathbb{G} = G(C, p)$ is an Erdős–Rényi graph with $H$ nodes and $p$ probability of connection between any two nodes.
\end{proof}
\end{lemma}

\cref{lemma:gossipconnectionprobability} allows us to compute the $\epsilon$-totality of \erg, given $G$.

\begin{theorem}
\label{theorem:ergtotality}
\erg\ satisfies $\epsilon_t$-totality, with $\epsilon_t$ bound by
\begin{equation}
    \label{equation:ergtotalitysecurity}
    \epsilon_t \leq \sum_{k = 1}^{C/2} \rp{{C \choose k}\rp{1 - p}^{k\rp{C - k}}}
\end{equation}
\begin{proof}
It follows immediately from \cref{lemma:gossipconnectionprobability} and a known result \cite{phasetransitions} on the connectivity of Erdős–Rényi graphs.
\end{proof}
\end{theorem}

\cref{figure:ergsecurity} shows the $\epsilon$-security of \erg, as a function of the gossip sample size ($G$), the fraction of Byzantine failures ($f$) and the size of the system ($N$).
