# Supplementary material for: AT2: Asynchronous Trustworthy Transfers
Source: arXiv:1812.10844 source file (2019-03-05)
Supplement: Supplementary file 2 [file shmem.tex]

%!TEX root = ../../main.tex

% \appendix

\section{Consensus number of a Payment System}
\label{app:consnum}

\subsection{System model}
\label{app:system-model}

\myparagraph{Processes and cryptographic primitives.}
We consider a set $\Pi$ of $N$ asynchronous processes that communicate through
reliable message-passing.
Every process is provided with a private-public key pair.

\myparagraph{Object types.}
A sequential object type is defined as a tuple
$T=(Q,q_0,O,R,\Delta)$, where $Q$ is a set of states, $q_0\in Q$ is an
initial state, $O$ is a set of operations, $R$ is a set responses and
$\Delta\subseteq Q\times O \times Q \times R$ is a relation
that associates a state and an operation to a set of
possible new states and corresponding responses.
Here we assume that $\Delta$ is total on the first two elements,
i.e., for each state $q\in Q$ and each operation in $o\in O$, some
transition to a new state is defined, i.e., $\exists q'\in Q,\; r\in
R$: $(q,o,q',r)\in \Delta$.

A \emph{history} is a sequence of invocations and responses and a
sequential history is a history that starts with an invocation and in
which every invocation is immediately followed with a response.
A \emph{sequential history} $o_1,r_1,o_2,r_2,\ldots$, where $\forall i\ge
1, o_i\in O,\; r_i\in R$, is \emph{legal} with respect to type
$T=(Q,q_0,O,R,\Delta)$ if there exists a
sequence of states $q_1,q_2,\ldots$ of states in $Q$ such that
$\forall i\geq 1$, $(q_{i-1},o_1,q_i,r_i)\in \Delta$.
%The \emph{sequential specification} of $T$ is the set of all sequential
%histories it accepts.

\myparagraph{Implementations.}
An \emph{implementation} of an object type $T$ is a distributed algorithm that,
for each process and invoked operation, prescribes the actions that the process needs to
take to perform it.
%In our case, the actions are accesses to shared atomic objects or   \textit{broadcast}
%primitives, processing of \textit{receive} events and returning
%responses to the invoked operations.
%
An \emph{execution} of an implementation is a sequence of
\emph{events}: invocations and responses of operations, \emph{send}
and \emph{receive} events, or atomic accesses to shared abstractions. The sequence of events at every process
must respect the algorithm assigned to it.
%A process is called \emph{faulty} in an infinite execution if
%stops before performing an event prescribed by its algorithm;
%otherwise it is called \emph{correct}.

%In the implementation, every process $p_i$ is assigned with an \emph{algorithm} $A_i$, an
%automaton that defines the actions $p_i$ needs to perform when it
%receives an input from its application or receives a message from
%another process.

\myparagraph{Failures.}
Processes are subject to \emph{Byzantine} failures. A process is
Byzantine if it deviates from the algorithm it is assigned, either by
halting prematurely, in which case we say that the process is \emph{crashed}, or performing actions
that are not prescribed by its algorithm, in which case we say that
the process is \emph{malicious}.
We assume that malicious processes can perform arbitrary actions,
except for ones that involve subverting cryptographic primitives (e.g. inverting secure hash functions).

A process is called \emph{faulty} if it is either crashed or malicious.
A process is \emph{correct} if it is not faulty and
\emph{benign} if it is not malicious. Note that every correct process
is benign, but not necessarily vice versa.

In a system with Byzantine processes, we assume that a fraction of less than $N/3$ processes can be malicious.

\myparagraph{Linearizability and sequential consistency.}
We assume that no process invokes a new operation before receiving a
response for the previous one.
For each pattern of invocations, the implementation produces a
\emph{history}, i.e., the sequence of distinct invocations and responses,
labelled with process identifiers and unique sequence numbers.

A projection of a history $H$ to process $p$, denoted $H|p$ is the
subsequence of elements of $H$ labelled with $p$.
An invocation $o$ by a process $p$ is \emph{incomplete} in $H$ if it is not followed by a
response in $H|p$.
A history is \emph{complete} if it has no incomplete invocations.
A \emph{completion} of $H$ is a history $\bar H$ that is identical to
$H$ except that every incomplete invocation in $H$ is either removed or
\emph{completed} by inserting a matching response somewhere after it.

A \emph{sequentially consistent} implementation of $T$ ensures that for every
history $H$ it produces, there exists a completion $\bar H$ and a
legal sequential history $S$ such that for all processes $p$, $\bar H|p=S|p$.
%In other words, the operations in $H$ are consistent to
%legal sequential history

A \emph{linearizable}  implementation, additionally, preserves the
real-time order between operations.
Formally, an invocation $o_1,r_1$ \emph{precedes} an
invocation $o_2$ in $H$, denoted  $o_1\prec_H o_2$, if $o_1$ is
complete and the corresponding response $r_1$ precedes $o_1$ in $H$.
Note that $\prec_H$ stipulates a partial order on invocations in $H$.
A linearizable implementation of $T$ ensures that for every history $H$ it produces, there exists a completion $\bar H$ and a
legal sequential history $S$ such that (1)~for all processes $p$, $\bar H|p=S|p$ and (2)~$\prec_H\subseteq\prec_S$.

A (sequentially consistent or linearizable) implementation is
\emph{$t$-resilient} if, under the assumption that at most $t$
processes crash, it ensures that every invocation performed by a
correct process is eventually followed by a response.
In the special case when $t=n-1$, we say that the implementation is
\emph{wait-free}.

In reasoning about correctness of an implementation, we cannot impose
restrictions on the behavior of malicious processes.
Thus, in the system with malicious processes,
given an object type, a history $H$ is \emph{sequentially consistent}
if there exists a
legal sequential history $S$ such that for all \emph{benign} processes $p$, $H|p=S|p$.
Note that $S$ may include arbitrary entries coming from malicious
processes.
%\pknote{Distinguish between honest (benign) and malicious?}
Similarly, a history is \emph{linearizable}
if it is sequentially consistent and $S$
respects the precedence order among operations issued by benign processes.
%\pknote{Prove that no linearizable algorithm exists with $f\geq n/2$?}

\myparagraph{Consensus number.}
In the  \emph{consensus} problem, each process starts with a private
\emph{input} value and is expected to decide on an \emph{output}
value, so that the following three properties are satisfied:
\begin{enumerate}
\item[(1)] no two processes decide on different output values,
\item[(2)] every decided output is an input of some process, and
\item[(3)] every correct process eventually decides on an output.
 \end{enumerate}

The \emph{consensus number} of a type $T$ is the maximal number of processes
that can (wait-free) solve consensus using atomic (linearizable) objects
of type $T$ and atomic registers.
For example, the consensus number of the \textsf{register} type is
one: even two processes cannot solve consensus using only
registers~\cite{FLP85,LA87}.

\subsection{Object Type of a Payment System}
\label{app:obj-type}

The \textsf{payment system} object type
%associated with a set of \emph{accounts} $\A$
is defined as a tuple $(Q,q_0,O,R,\Delta)$, where:

\begin{itemize}

\item The set of states $Q$ is the set of all possible maps
  $q:\;\Pi\to\Nat$. Intuitively, each state of the objects assigns
  each account with its \emph{balance}.

\item The initialization map  $q_0:\;\Pi\to\Nat$ assigns the initial
  balance to each account. We assume the initialization map to be fixed for the rest
  of the paper.

\item Operations and responses of  the type are defined as $O=\{\textit{pay}(a,b,x):\; a,b\in\Pi,\,
  x\in\Nat\}\cup\{\textit{read}(a):\;a\in\Pi\}$ and
  $R=\{\true,\false\}\cup\Nat$.

 \item For a state $q\in Q$, an operation $o\in O$, a response
   $r\in R$ and a new state $q'\in Q$, the tuple $(q,o,q',r)\in\Delta$
   if and only if one of the following conditions is satisfied:

  \begin{itemize}

     \item $o=\textit{pay}(a,b,x)$: $q(a)\geq x$, $q'(a)=q(a)-x$, $q'(b)=q(b)+x$ (and all other
       accounts are as in $q$), and $r=\true$;

     \item $o=\textit{pay}(a,b,x)$: $q(a)< x$, $q'=q$, and $r=\false$;

     \item o=$\textit{read}(a)$: $q=q'$, $r=q(a)$.

   \end{itemize}

  \end{itemize}

In other words, operation $\textit{pay}(a,b,x)$ \emph{succeeds} if and only if the source
account $a$  has enough balance, and if it does, $x$ is transferred
from $a$ to the destination account $b$.
An $\textit{pay}(a,b,x)$ operation is called \emph{outgoing} for
$a$ and \emph{incoming} for $b$; respectively, the $x$ units are called   \emph{outgoing} for
$a$ and \emph{incoming} for $b$.
A transfer is \emph{successful} if its corresponding response is \emph{true} and \emph{failed} if its corresponding response is \emph{false}.

Operation $\textit{read}(a)$ simply returns the balance of $a$ and
leaves the accounts untouched.

%Let $\mu:\;\Pi\to\Pi$ be the \emph{ownership map} associating each account with a distinct
%process. We require that only $\mu(a)$, the owner of account $a\in \Pi$, is
%allowed to perform $\textit{pay}$ operations on it.
%
%% In a system in which all processes are benign (correct or failing by
%% crashing), we assume that a process $p$ invokes
%% $\textit{pay}(a,.,.)$ or $\textit{read}(a)$ only if $a=p$.
%% Further, in a system assuming the presence of malicious processes, the
%% requirement only applies to benign processes.
%
We assume that every benign process $p$ is \emph{well-formed}: (1)~it
only invokes operations $\textit{read}(a)$ and
$\textit{pay}(a,*,*)$ such that $a=p$ and (2)~it never invokes a new operation before obtaining a response from a previous one.

While not requiring malicious processes to be well-formed, a cryptographic proof of a process invoking an operation on an
account that the process does not own can be used as a proof of misbehavior.

%% \subsection{Banking in a Byzantine environment}
%% %

%% \needsrev{
%% We discuss two implementations of the \textsf{banking} data type.
%% %
%% The first one is a conventional linearizable implementation.
%% %
%% The second one ensures sequential consistency for \emph{updates}, i.e.,
%% successful pay operations and a specific level of \emph{stale}
%% consistency for \emph{read-only} operations, i.e., reads and
%% failed transfers.
%% }

\subsection{Consensus Number of Payment System}
\label{app:consensus-number}

We show that the \textsf{payment system} object type can be
implemented in the \emph{wait-free} manner using only read-write
registers.
Thus, the type is of consensus number $1$.

The implementation is described in Figure~\ref{fig:waitfree}.
The idea is very simple.
The $n$ processes share an atomic snapshot object~\cite{atomic-snapshot}.
Every process $p$ is associated with a distinct location in the object
where it stores the sequence of all successful {\transfer} operations
it executed so far.

Recall that the atomic-snapshot (AS) memory is represented as a vector of $n$
shared variables, where each process $p$ is associated with a distinct
position $p$. The memory can be accessed with two atomic operations: \emph{update} and
\emph{snapshot}. An \emph{update} operation performed by $p$
modifies the value at position $p$  and a \emph{snapshot} returns the current state of the vector.

To read the balance of an account $a$, the process simply takes a snapshot $S$ and
computes the sum of incoming units minus the sum of all outgoing
units, we  denote this number by $\textit{balance}(a,S)$.
As we argue below, the result is guaranteed to be non-negative,
i.e., the operation does make sense with respect to the type specification.

To perform $\transfer(a,b,x)$, a process $p$, the owner of $a$, takes a snapshot and
computes the balance of $a$ based on all operations that
\emph{concern} $a$ (transfer units from or to $a$).
If the amount to be transferred does not exceed the balance of $a$
computed based on operations in the snapshot, the operation is added
to the list of $p$'s operations in the snapshot object via an
\textit{update} operation and $\true$ is returned.
Otherwise, the operation returns $\false$.

Note that security concerns are not central for us now.
In particular, every process has a complete view of all the accounts,
regardless of whether it owns them or not.

\begin{theorem}
  \label{th:waitfree}
  The \textsf{payment system} object type can be wait-free implemented in the
  read-write shared memory model.
\end{theorem}
\begin{proof}
  Fix an execution $E$ of the algorithm in Figure~\ref{fig:waitfree}.
   As, atomic snapshots can be wait-free implemented in the read-write
   shared memory model~\cite{atomic-snapshot}.
  As every operation only involves a finite number of atomic-snapshot
  accesses, every process completes each of the operations it invokes
  in a finite number of its own steps.

Let $\textit{Ops}$ be union of all complete operations and
all {\transfer} operations that \emph{completed} the update operation
(line~\ref{line1:tsf:update}) in $E$ (the atomic snapshot operation
has been linearized).
Let $H$ be the history of $E$.
We determine a completion of $H$ and, for each $o\in\textit{Ops}$, we define a linearization point as
`follows:

\begin{itemize}

  \item If $o$ is a {\read} operation, it linearizes at the
    linearization point of the snapshot operation in
    line~\ref{line1:read:snapshot}.

  \item   If $o$ is a {\transfer} operation that returns {\false},
    it linearizes at the linearization point of the snapshot operation in
    line~\ref{line1:tsf:snapshot}.

 \item   If $o$ is a {\transfer} operation completed in
   line~\ref{line1:tsf:update},  it linearizes at the
    linearization point of the update operation in
    line~\ref{line1:tsf:update}.
    If $o$ is incomplete in $H$, we complete it with response $\true$.

\end{itemize}

Let $\bar H$ be the resulting complete history and let $L$ be sequence
of complete operations of $\bar H$ places in the order of their
linearization points in $E$.
Note that, by the way we linearize operations, the linearization of a
prefix of $E$ is a prefix of $L$.

Now we show that $L$ is legal and, thus, $H$ is
linearizable.
We proceed by induction, starting with the empty (trivially, legal)
prefix of $L$.
Let $L_{\ell}$ be the legal prefix of the first $\ell$ operation and
$op$ be the $(\ell+1)$st operation of $L$.
Let $op$ be invoked by process $p$.
The following cases are possible:

\begin{itemize}

\item $op$ is a {\read}$(a)$: the snapshot taken at the linearization point of $op$
  contains all successful payments concerning $a$ in $L_{\ell}$. By
  the induction hypothesis, the resulting balance is non-negative.

\item $op$ is a failed {\transfer}$(a,b,x)$: the snapshot taken at the linearization point of $op$
  contains all successful payments concerning $a$ in $L_{\ell}$. By
  the induction hypothesis, the resulting balance is non-negative.

\item  $op$ is a successful  {\transfer}$(a,b,x)$:  by the algorithm,
  before the linearization point of $op$, process $p$ took a snapshot.
  Let $L_{k}$, $k\leq\ell$, be the prefix of $L_{\ell}$ that only
  contain operations linearized before the moment of time when the
  snapshot was taken by $p$.

  We observe that includes a \emph{subset} of all incoming payments on $a$ and
  \emph{all} outgoing payments on $a$ in $L_{\ell}$. Indeed, as $p$
  is the owner of $a$ and only the owner of $a$ can perform outgoing
 payments on $a$, all outgoing payments in $L_{\ell}$ were
  linearized before the moment $p$ took the snapshot within $op$.
  Thus, $\textit{balance}(a,L_k)\geq \textit{balance}(a,L_{\ell})$.

  By the algorithm, as $op={\transfer}(a,b,x)$ succeeds, we have
  $\textit{balance}(a,L_k)\geq x$.
  Thus, $\textit{balance}(a,L_{\ell})\geq x$ and the resulting balance
  in $L_{\ell+1}$ is non-negative.

\end{itemize}

Thus $H$ is linearizable.
\end{proof}

\begin{corollary}\label{cor:consensus}
The \textsf{payment system} object type has consensus number $1$.
\end{corollary}

\section{Defining a Byzantine Fault-Tolerant Payment System}
\label{app:byz}

In the message-passing context with Byzantine processes, we propose a
relaxed consistency definition that will allow us to build an
efficient implementation.
The implementation ensures linearizability to successful pay
operations, while reads and failed payments are provided with a
weaker consistency property.
Intuitively, every operation performed by a benign process $p$ that does not change the state of the banking object
is consistent with the ever-growing $p$'s local history\footnote{The \emph{local history} of a process $p$ is the subset of the global history observed by $p$.} which might
possibly miss some of the complete incoming payments.
One can argue that this relaxation incurs very little impact on the
utility of the banking application, as long as all incoming payments
are \emph{eventually} accounted for.

%Intuitively, by doing so we relax
%the requirement that complete operations \emph{take effect} in their
%precedence order. It can be argued that the requirement is not central
%for banking applications.

More precisely, we require that in every history $H$ produced by the implementation,
each correct process completes all of its operations.
Moreover, we expect that the \emph{successful} payments in $H$ are
compatible with the same legal sequential execution. In particular, regardless of the
behavior of Byzantine processes, we exclude the problem of double
spending: there is no way a faulty process can spend more money than
its account allows.
Additionally, we require that
reads and unsuccessful payments performed by every benign process $p$ are
compatible with \emph{some} (possibly depending on the process) legal
sequential history.
Also, if $p$ and $q$ are correct, then every successful payment from
$p$ to $q$ is eventually included in $q$'s local history.
%All operations of $p_i$ ``make sense'' for some
%ordering of operations $H$.

\begin{definition}
\label{def:banking-relaxed}
 Let $E$ be any execution of an implementation and $H$ be
the corresponding history.
Let $\textit{ops}(H)$ denote the set of operations in $H$ that were
executed by correct processes in $E$.
A \emph{relaxed} banking object guarantees that
each invocation issued by a correct process is followed by a
matching response in $H$, and that there exists $\bar H$,  a completion of $H$, such that:

\begin{enumerate}

\item[(1)] Let $\bar H^{t}$ denote the sub-history of
  successful payments of $\bar H$ performed by correct processes and
  $\prec_{\bar H}^t$ be the subset of $\prec_{\bar H}$ restricted to
  operations in $\bar H^{t}$.
  %we call such a history
%\emph{transfer-only}.
  Then there exists a legal sequential history $S$ such that (a)~for every correct process
$p$, $\bar H^{t}|p=S|p$ and (b)~$\prec_{\bar H}^t\subseteq\prec_S$.
 %with respect to the
 % specification of \textsf{banking}.

\item[(2)] For every correct process $p$, there exists a legal sequential history $S_p$
  such that:

  \begin{itemize}

  \item $\textit{ops}(\bar H) \subseteq \textit{ops}(S_p)$, and

  \item $S_p|p= \bar H |p$.

  \end{itemize}

\end{enumerate}
\end{definition}

Notice that property~(2) implies  that every update in $H$ that
affects the account of a correct process $p$ is eventually included in
$p$'s ``local'' history and, therefore, will reflect
reads and pay operations subsequently performed by $p$.
%[[PK already said
%It is possible, however, that $p_i$ may temporarily miss some of the
%transfers affecting its accounts and, as a result, local views of
%different accounts may not be compatible with the same sequential
%history.
%]]
